# Supplementary material for: The Effect of Alignment Objectives on Code-Switching Translation
Source: arXiv:2309.05044 source file (2023-09-10)
Supplement: Supplementary file 1 [file 09-appendicies.tex]

\appendix

\section{Appendix}
\label{AppendixA}
